# Supplementary material for: Whole-Herd Elephant Pose Estimation from Drone Data for Collective Behavior Analysis
Source: arXiv:2411.00196 source file (2024-10-31)
Supplement: Supplementary file 1 [file supplementary_smallds_dlc.tex]

% Side experiment -- smaller training dataset.  I will omit for now
%To train DeepLabCut, two methods were explored. In the first, 5 frames from each video were selected using K-means quantization-based extraction \cite{Vector2023} and were manually annotated with the keypoints shown in Figure 1. This results in a training dataset of 105 labeled pose patches. DeepLabCut was fine-tuned on this dataset for 100 epochs. DeepLabCut is known for its efficiency with small datasets, so this dataset size may be sufficient \cite{Mathis2018-jg}. 

% ok I'll omit this but here's the values for it's performance in this table.. the val and the test are for these nets. 
% This network works well on val (same video, different frame) but poorly on test. It's worth noting though cause it's a 100 labels instead of 1400, so that's nice.. 

\begin{table*}[ht]
    \centering
    \begin{tabular}{cccccccccc} % Seven columns, all centered
        \hline
        & \multicolumn{3}{c}{DeepLabCut (Val) } & \multicolumn{3}{c}{DeepLabCut (Test) } & \multicolumn{3}{c}{YOLO-NAS-Pose} \\
        \hline
        & RMSE & PCK & OKS & RMSE & PCK & OKS & RMSE & PCK & OKS \\ % Header row
        \hline
        forehead & 2.43 & 64.7 & 0.81 & 35.4 & 1.50 & 0.05 & 20.12 & 0.0 & 0.02 \\    % Data row 1
        ear\_base\_l & 2.16 & 76.4 & 0.85 & 1.50 & 6.01 & 0.08 & 3.11 & 68.7 & 0.84 \\    % Data row 2
        ear\_base\_r & 2.29 & 70.6 & 0.84 & 26.4 & 3.01 & 0.07 & 2.34 & 63.9 & 0.85 \\    % Data row 3
        skull\_base & 1.99 & 58.8 & 0.86 & 23.1 & 3.76 & 2.98 & 0.08 & 64.5 & 0.82 \\    % Data row 4
        shoulders & 2.63 & 23.6 & 0.77 & 11.8 & 5.26 & 3.94 & 0.16 & 40.4 & 0.72 \\    % Data row 5
        hips & 4.32 & 17.6 & 0.59  & 34.4 & 0 & 0.02 &3.22 & 67.5 & 0.82 \\    % Data row 6
        ear\_tip\_l & 2.88 & 47.1 & 0.76 & 21.9 & 3.00 & 0.08 & 3.50 & 47.0 & 0.75 \\    % Data row 7
        ear\_tip\_r & 3.07 & 35.3 & 0.72 & 20.2 & 3.76 & 0.06 & 3.36 & 53.6 & 0.75 \\    % Data row 8
        Average & \textbf{2.72} & \textbf{49.3} & \textbf{0.78} & \textbf{25.0} & \textbf{3.29} & \textbf{0.07} & \textbf{5.32} & \textbf{50.7} & \textbf{0.70} \\ % Data row 9
        \hline
    \end{tabular}
    \caption{Performance metrics of DeepLabCut and YOLO-NAS-Pose models on the test set. Due to the low performance of DeepLabCut on the test set, the validation set was also included.}
    \label{tab:pose_metrics}
\end{table*}

% discussion 
DeepLabCut, when compared to YOLO-NAS-Pose, exhibited signs of severe overfitting, as evidenced by the discrepancy between its performance on validation and test metrics.

While DeepLabCut demonstrated satisfactory qualitative results in labeling a full video from the validation set—where only a few frames were part of the training data—the overfitting issue remains significant. The validation and training datasets were composed of mixed frames from the same videos, leading to an over-generalization to those specific scenarios. 

However, in similar but distinct environments, DeepLabCut struggled. To mitigate this, future work should ensure that training and validation datasets are derived from different videos and locations, enhancing the network's ability to generalize.
